# Supplementary material for: Study of the doubly charmed tetraquark $T_{cc}^+$
Source: arXiv:2109.01056 source file (2022-06-16)
Supplement: Supplementary file 1 [file supplementary-CDS.tex]

\setcounter{figure}{0}
 \setcounter{table}{0}
 \setcounter{equation}{0}
 
\section*{Supplementary material for LHCb-PAPER-2021-032}
\label{sec:supplementary}

%% This appendix contains supplementary material that will be posted
%% on the public CDS record but will not appear in the paper.

\subsection*{Summary of theory predictions}
Theory predictions for the~mass of the~ground isoscalar $\mathrm{J^P=1^+}$
  tetraquark \Tcc state are summarised in Fig.~\ref{fig:predicttions}.

\begin{figure}[htb]
  \setlength{\unitlength}{1mm}
  \centering
  \begin{picture}(150,182)
    %% 
    %% \graphpaper[5](-10,-10)(170,200)
    %% 
    \put( 0, 0){ 
      \includegraphics*[height=180mm,%
      %% ]{DATA_Gamma0_profile2.pdf}
      %%]{DATA_BWU_profile_gamma0.pdf} 
      %% ]{theory1.pdf}
      ]{theory9.pdf}
    }
    %% 
    %% \put(74,93){\scriptsize\begin{Tabular}[1.51]{lcc}
    \put(72,93){\footnotesize\begin{Tabular}[1.20]{lcc}
   %% 
    %% J.~Carlson, L.~Heller and J.~A.~Tjon & \cite{Carlson:1987hh} & 1987
    J.~Carlson \etal  & 1987 & \cite{Carlson:1987hh} 
    \\
    B.~Silvestre-Brac and C.~Semay & 1993 & \cite{SilvestreBrac:1993ss}
    \\
   C.~Semay and B.~Silvestre-Brac & 1994 & \cite{Semay:1994ht} 
    \\
    %% M.~A.~Moinester & \cite{Moinester:1995fk} & 1995 & $-276$ 
     M.~A.~Moinester & 1995 & \cite{Moinester:1995fk}
    \\
   %% S.~Pepin, F.~Stancu, M.~Genovese and J.~M.~Richard & \cite{Pepin:1996id} & 1996 
    S.~Pepin \etal  & 1996 & \cite{Pepin:1996id} 
  \\
   B.~A.~Gelman and S.~Nussinov & 2003 & \cite{GELMAN2003296} 
   \\
    %% J.~Vijande, F.~Fernandez, A.~Valcarce, A. and B.~Silvestre-Brac
    %% & \cite{Vijande:2003ki} & 2003 
     J.~Vijande \etal  & 2003 & \cite{Vijande:2003ki}
  \\
   D.~Janc and  M.~Rosina & 2004 & \cite{Janc:2004qn}
   \\  
  %% F.~Navarra, M.~Nielsen and S.~H.~Lee & \cite{Navarra:2007yw} & 2007
    F.~Navarra \etal & 2007 & \cite{Navarra:2007yw}
    \\
   %% J.~Vijande, E.~Weissman, A.~Valcarce & \cite{Vijande} & 2007 
   J.~Vijande \etal & 2007 & \cite{Vijande} 
   \\
  %% D.~Ebert, R.~N.~Faustov, V.~O.~Galkin and W.~Lucha & \cite{Ebert:2007rn} & 2007 & $+60\phantom{0}$
   D.~Ebert \etal & 2007 & \cite{Ebert:2007rn} 
   \\ 
   S.~H.~Lee and S.~Yasui & 2009 & \cite{Lee:2009rt} 
  \\
  %% Y.~Yang, C.~Deng, J.~Ping and T.~Goldman & \cite{Yang2009} & 2009 & $+88$ 
   Y.~Yang \etal & 2009 & \cite{Yang2009}
  \\
  %% N.~Li, Z.\nobreakdash-F.~Sun, X.~Liu  and S.\nobreakdash-L.~Zhu  &
  N.~Li \etal & 2012 & \cite{Li:2012ss}
  \\
  %% G.-Q.~Feng, X.-H.~Guo and B.-S.~Zou & \cite{Feng:2013kea} & 2013
  G.-Q.~Feng \etal & 2013 & \cite{Feng:2013kea}
  \\
  %% Y.~Ikeda, B.~Charron, S.~Aoki, 
  %% T.~Doi, T.~Hatsuda, T.~Inoue, 
  %% N.~Ishii, K.~Murano, H.~Nemura and K.~Sasaki 
  %% & \cite{Ikeda:2013vwa} & 2013  & $[-70,+124]$ 
  %% Y.~Ikeda \etal  & 2013 & \cite{Ikeda:2013vwa} 
  %% \\
  %% S.-Q.~Luo, K.~Chen, X.~Liu, Y.-R.~Liu and S.-L.~Zhu & \cite{Luo:2017eub} & 2017 
  %% & 
  %% %% $-96\phantom{0}$ 
  %% $+100$
  S.-Q.~Luo \etal & 2017 & \cite{Luo:2017eub} 
  \\
  M.~Karliner and J.~Rosner & 2017 & \cite{Karliner:2017qjm} 
  \\
   E.~J.~Eichten and C.~Quigg & 2017 & \cite{Eichten:2017ffp} 
  \\
  Z.~G.~Wang & 2017 & \cite{Wang:2017uld} 
  \\    
 %% %% G.~K.~C.~Cheung, C.~E.~Thomas, J.~J.~Dudek and R.~G.~Edwards 
 %% & \cite{Cheung:2017tnt} & 2017 & $ %% \lesssim 0 $ 
 %% G.~K.~C.~Cheung \etal & 2017 & \cite{Cheung:2017tnt}
 %% \\
  %% W.~Park,   S.~Noh and S.~H.~Lee & \cite{Park:2018wjk} & 2018  
  W.~Park \etal & 2018 & \cite{Park:2018wjk} 
\\
 %%  %% A.~Francis, R.~J.~Hudspith, R.~Lewis  and K.~Maltman & 
 %% \cite{Francis:2018jyb} &  2018 & $\sim0$
 %% A.~Francis \etal & 2018 & \cite{Francis:2018jyb} 
 %% \\
  %% P.~Junnarkar, N.~Mathur and M.~Padmanath & \cite{Junnarkar:2018twb} & 2018 
   P.~Junnarkar \etal & 2018 & \cite{Junnarkar:2018twb}
  \\
  %% C.~Deng, H.~Chen and J.~Ping & \cite{Deng:2018kly} &   2018
  C.~Deng \etal & 2018 & \cite{Deng:2018kly} 
 \\
   %% M.-Z.~Liu, T.-W.~Wu,  V.~Pavon Valderrama, J.-J.~Xie and  L.-S.~Geng
  %% & \cite{Liu:2019stu}
  %% & 2019 
  %% & $-3^{+4}_{-15}$ 
   M.-Z.~Liu \etal  & 2019 & \cite{Liu:2019stu} 
  \\
  %% L.~Maiani, A.~Polosa and V.~Riquer 
  %% & \cite{Maiani:2019lpu}
  %% & 2019 
  %% & $\left[-10,+7]\right]$ 
  L.~Maiani \etal & 2019 & \cite{Maiani:2019lpu}
  \\
  %% G.~Yang,   J.~Ping and J.~Segovia &   \cite{Yang:2019itm} & 2019 
  G.~Yang \etal &  2019 &  \cite{Yang:2019itm} 
\\
 %% Y.~Tan, W.~Lu and J.~Ping & \cite{Tan:2020ldi} & 2020 
  Y.~Tan \etal  & 2020 & \cite{Tan:2020ldi} 
 \\   
  %% Q.-F.~L\"u, D.-Y.~Chen   and Y.-B.~Dong & \cite{Lu:2020rog} & 2020 
  Q.-F.~L\"u \etal  & 2020 & \cite{Lu:2020rog}  
 \\
 %% E.~Braaten,  L.-P.~He   and A.~Mohapatra & \cite{Braaten:2020nwp} & 2020 
  E.~Braaten \etal & 2020 & \cite{Braaten:2020nwp} 
 \\
 %% D.~Gao , D.~Jia, Y.-J.~Sun, Z.~Zhang,
  %%  W.-N.~Liu and Q.~Mei 
  %% & \cite{Gao:2020ogo} & 2020 & $\left[-250,+2\right]$
  D.~Gao \etal & 2020 & \cite{Gao:2020ogo} 
  \\
  %% J.-B.~Cheng, S.-Y.~Li, Y.-R.~Liu, Z.-G.~Si, T.~Yao & \cite{Cheng:2020wxa} & 2020 & $+53\phantom{0}$ 
  J.-B.~Cheng \etal & 2020 & \cite{Cheng:2020wxa} 
  \\
  %% S.~Noh,  W.~Park and S.~H.~Lee & \cite{Noh:2021lqs} & 2021
  S.~Noh \etal  & 2021 & \cite{Noh:2021lqs} 
  \\
  %% R.~N.~Faustov, V.~O.~Galkin and E.~M.~Savchenko 
  R.~N.~Faustov \etal & 2021 & \cite{Faustov:2021hjs} 
 \end{Tabular}}
    \put( 35,2){\large$\updelta m$}
    \put( 53,2){\large$\left[\!\mevcc\right]$ }
    \put(12,179){\large$\updelta m_{\mathrm{U}}
    = -359\pm 40 {}^{\,+\,9}_{\,-\,6} \kevcc$}
  \end{picture}
  \caption {\small
  Theory predictions 
  for the~mass of the~isoscalar $\mathrm{J^P=1^+}$
  $\cquark\cquark\uquarkbar\dquarkbar$~tetraquark 
  \Tcc~ground state~\cite{Carlson:1987hh,
SilvestreBrac:1993ss,
Semay:1994ht,
Moinester:1995fk,
Pepin:1996id,
GELMAN2003296,
Vijande:2003ki,
Janc:2004qn,
Vijande,
Navarra:2007yw,
Ebert:2007rn,
Lee:2009rt,
Yang2009,
Li:2012ss,
Feng:2013kea,
%% Ikeda:2013vwa,
Eichten:2017ffp,
Karliner:2017qjm,
%% Cheung:2017tnt,
Luo:2017eub,
Wang:2017uld,
Deng:2018kly,
%% Francis:2018jyb,
Junnarkar:2018twb,
Park:2018wjk,
Liu:2019stu,
Maiani:2019lpu,
Yang:2019itm,
Cheng:2020wxa,
Lu:2020rog,
Braaten:2020nwp,
Tan:2020ldi,
Gao:2020ogo,
Noh:2021lqs,
Faustov:2021hjs}.
Masses are shown 
relative to the~\Dstarp\Dz~mass threshold.
}
  \label{fig:predicttions}
\end{figure}
