# Supplementary material for: Study of the doubly charmed tetraquark $T_{cc}^+$
Source: arXiv:2109.01056 source file (2022-06-16)
Supplement: Supplementary file 2 [file supplementary.tex]

\pdfoutput=1
% Uncomment line above if submitting to arXiv and using pdflatex
% ============================================================================
% Purpose: Template for LHCb documents
% Authors: Tomasz Skwarnicki, Roger Forty, Ulrik Egede, Patrick Koppenburg
% Created on: 2010-09-24
% ============================================================================
\documentclass[12pt,a4paper]{article}
%%\documentclass[12pt,letter]{article}
% For two column text, add "twocolumn" as an option to the document
% class. Also uncomment the two "onecolumn" and "twocolumn" lines
% around the title page below.

% Variables that controls behaviour
\usepackage{ifthen} % for conditional statements
\newboolean{pdflatex}
\setboolean{pdflatex}{true} % False for eps figures 

\newboolean{articletitles}
\setboolean{articletitles}{true} % False removes titles in references

\newboolean{uprightparticles}
\setboolean{uprightparticles}{true} %True for upright particle symbols

%\newboolean{inbibliography}
%\setboolean{inbibliography}{false} %True once you enter the bibliography

% Define titles and authors here. It will then be used both in metadata and in
% what is printed on the front page.
 % Leave as is for PAPER, CONF and FIGURE
%% \def\paperasciititle{Observation of a narrow state near D*+D0 mass threshold} 
%% \def\papertitle{Observation of a~narrow state  
%% near $\Dstarp\Dz$~mass threshold} % Latex formatted title
%%
 
 % Latex formatted title
%%
 % Comma separated list
%\def\papercopyright{CERN on behalf of the LHCb collaboration}
\def\papercopyright{\the\year\ CERN for the benefit of the LHCb collaboration} % new since 9/Apr/2018

\usepackage{lscape}
\usepackage{comment}
\usepackage{graphpap} 
\usepackage{multirow} 
\usepackage{rotating} 
\usepackage{mathrsfs}
\usepackage{mathtools} %% dcases 
\usepackage{dashrule}
\usepackage{tikz}
\usepackage{enumerate}
\usepackage{enumitem}
\usetikzlibrary{patterns}
\usepackage{nicefrac} %% 1/2, ...
\usepackage{afterpage}
\usepackage{xcolor}
\usepackage[toc,page]{appendix}
\usepackage[normalem]{ulem} 
\usepackage{wasysym}

%% \makeatletter
%% \g@addto@macro\
%% \makeatother

\input{preamble}
\usepackage{longtable} % only for template; not usually to be used in PAPERs

\makeatletter
\g@addto@macro\bfseries{\boldmath}
\makeatother

\input{local-symbols}

\begin{document}

%% \numberwithin{equation}{section}
%% \numberwithin{table}{section}
%% \numberwithin{figure}{section}

%%%%%%%%%%%%%%%%%%%%%%%%%
%%%%% Title     %%%%%%%%%
%%%%%%%%%%%%%%%%%%%%%%%%%
%% \renewcommand{\thefootnote}{\fnsymbol{footnote}}
%% \setcounter{footnote}{1}

% %%%%%%% CHOOSE TITLE PAGE--------
%\onecolumn
%\input{title-LHCb-INT}
%\input{title-LHCb-ANA}
%\input{title-LHCb-CONF}
%\input{title-LHCb-FIGURE}
%\input{title-LHCb-PAPER}
%\twocolumn
% %%%%%%%%%%%%% ---------

\renewcommand{\thefootnote}{\arabic{footnote}}
\setcounter{footnote}{0}

%%%%%%%%%%%%%%%%%%%%%%%%%%%%%%%%
%%%%%  Table of Content   %%%%%%
%%%%%%%%%%%%%%%%%%%%%%%%%%%%%%%%
%%%% Uncomment if desired
%\tableofcontents
\cleardoublepage

%%%%%%%%%%%%%%%%%%%%%%%%%
%%%%% Main text %%%%%%%%%
%%%%%%%%%%%%%%%%%%%%%%%%%

\pagestyle{plain} % restore page numbers for the main text
\setcounter{page}{1}
\pagenumbering{arabic}

%% Uncomment during review phase. 
%% Comment before a final submission.
%% \linenumbers

\input{supplementary-NC}

\clearpage
\addcontentsline{toc}{section}{References}
%\setboolean{inbibliography}{true}
\bibliographystyle{LHCb}
\bibliography{main,standard,LHCb-PAPER,LHCb-CONF,LHCb-DP,LHCb-TDR}

\end{document}
